# Supplementary material for: Elastocapillary Snapping: Capillarity Induces Snap-Through Instabilities in Small Elastic Beams
Source: arXiv:1307.1775 source file (2014-04-07)
Supplement: Supplementary file 1 [file DropSnapping-suppmat.pdf]

## Supplementary information on ‘Elastocapillary Snapping’

Aurélie Fargette<sup>1,2,3</sup>, Sébastien Neukirch<sup>2,3</sup>, and Arnaud Antkowiak<sup>2,3</sup>

<sup>1</sup>*Département de Physique, École Normale Supérieure, 24 rue Lhomond, 75005 Paris, France.*

<sup>2</sup>*CNRS, UMR 7190, Institut Jean Le Rond d’Alembert, F-75005 Paris, France.*

<sup>3</sup>*UPMC Université Paris 06, UMR 7190, Institut Jean Le Rond d’Alembert, F-75005 Paris, France*

(Dated: July 5, 2013)

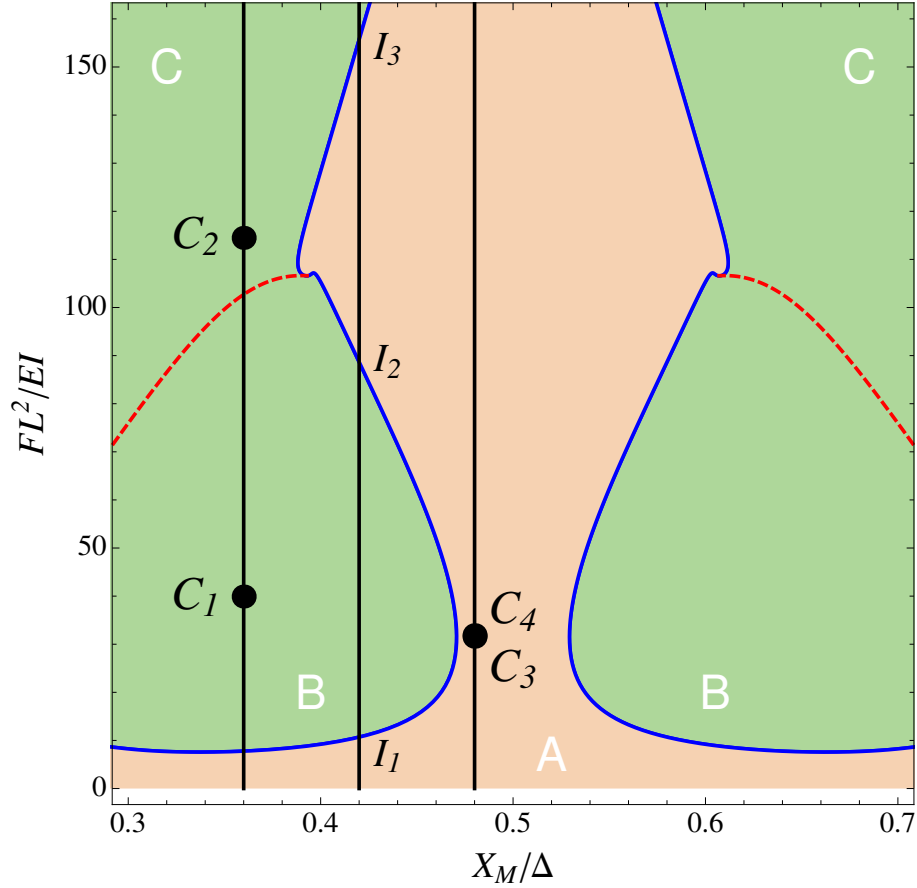

FIG. 1. Phase diagram as in Fig. 4(b) of main text, but with three additional vertical lines corresponding to  $x_M = 0.36\Delta$ ,  $x_M = 0.42\Delta$ , and  $x_M = 0.48\Delta$ .

#### BIFURCATION DIAGRAMS ASSOCIATED TO FIG. 4

We here show some bifurcation diagrams in relation to the phase diagram presented in Fig. 4 of the main text. As in other problems where capillarity, weight, and elasticity are present the following quantities are found to be relevant:

$$\begin{aligned} L_{eg} &= \sqrt{EI/(\lambda g)} \\ L_{ec} &= \sqrt{EI/(\gamma w)} \\ L_c &= \sqrt{\gamma/(\rho g)} \end{aligned}$$

Using parameters from Table 1, we find  $L_{eg} = 0.683 L$ ,  $L_{ec} = 0.0736 L$ , and  $L_c = 0.774 L$ . Nevertheless in the numerical computations we made use of an effective value  $\gamma_{\text{model}} = 0.67\gamma$ , thereby changing  $L_{ec}$  and  $L_c$  to  $L_{ec} = 0.09 L$  and  $L_c = 0.634 L$ . In Fig. 2 the bifurcation diagram for  $x_M = 0.36\Delta$  is drawn with points corresponding to  $C_1$  and  $C_2$  configurations. Configuration  $C_1$  (respectively  $C_2$ ) has  $Y_M > 0$  (resp.  $Y_M < 0$ ) and hence is called an upward (resp. downward) buckled configuration. Along the bifurcation curve, at  $FL^2/(EI) \simeq 100$ ,  $Y_M$  changes sign and this corresponds to the crossing of  $x_M = 0.36\Delta$  with the dotted curve in Fig. 1. In Fig. 3 we have plotted the three fold points  $I_{1,2,3}$ , that are also shown in Fig. 1. These points are instability points and correspond to the loss of stability of an equilibrium as one leaves the bistable region A in Fig. 1. In Fig. 4 we have plotted the two points  $C_3$  and  $C_4$ , corresponding to stables configuration having the same value of  $FL^2/(EI)$ . These points lie in the bistable region A that extends up to  $FL^2/(EI) \simeq 220$ . For larger  $F$  values only the downward buckled configuration remains (in upper region C, out of the range of Fig. 1).

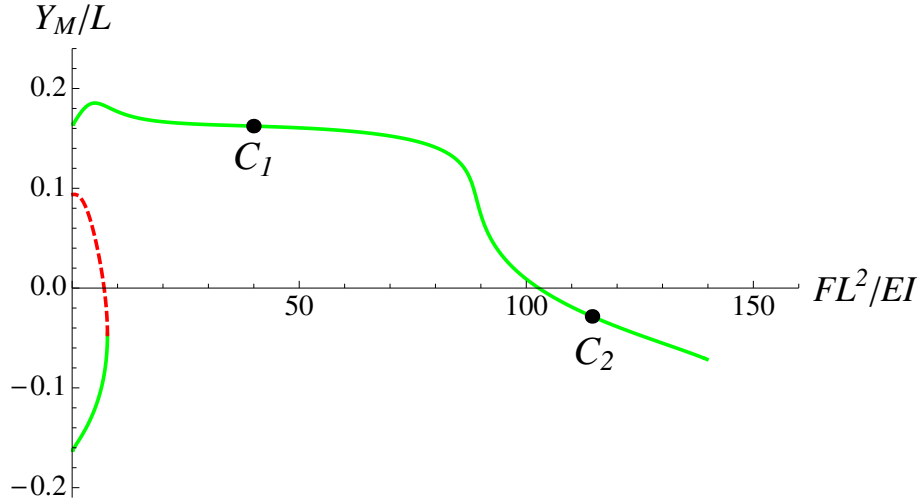

FIG. 2. Bifurcation diagram for  $x_M = 0.36\Delta$  showing  $C_1$  and  $C_2$  configurations. Plain (respectively dotted) curves correspond to stable (resp. unstable) equilibria.

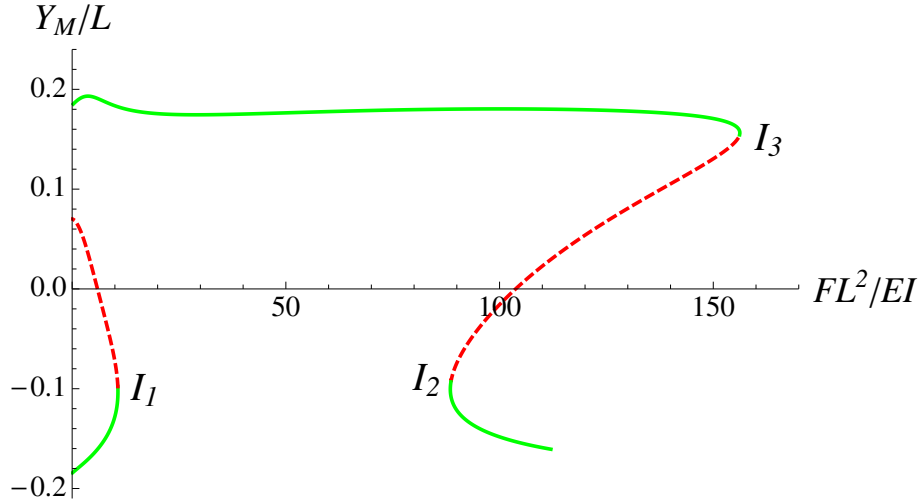

FIG. 3. Bifurcation diagram for  $x_M = 0.42\Delta$ . Plain (respectively dotted) curves correspond to stable (resp. unstable) equilibria. Also shown are the three fold points  $I_{1,2,3}$  where stability changes.

### SNAPPING DYNAMICS

The shape of the beam as it leaves the unstable equilibrium is recorded with a high-speed camera and the vertical position  $y_s(s = L/2, t)$  of the midpoint of the beam is extracted from the image sequence. From the fit

$$y_s(L/2, t) = y_0 + y_1 e^{\mu t} \quad (1)$$

we obtain the growth rate  $\mu$ . In Fig. 5 we plot  $y_s(s = L/2, t)$  together with three snapshots showing the instantaneous shape of the beam during the snapping event.

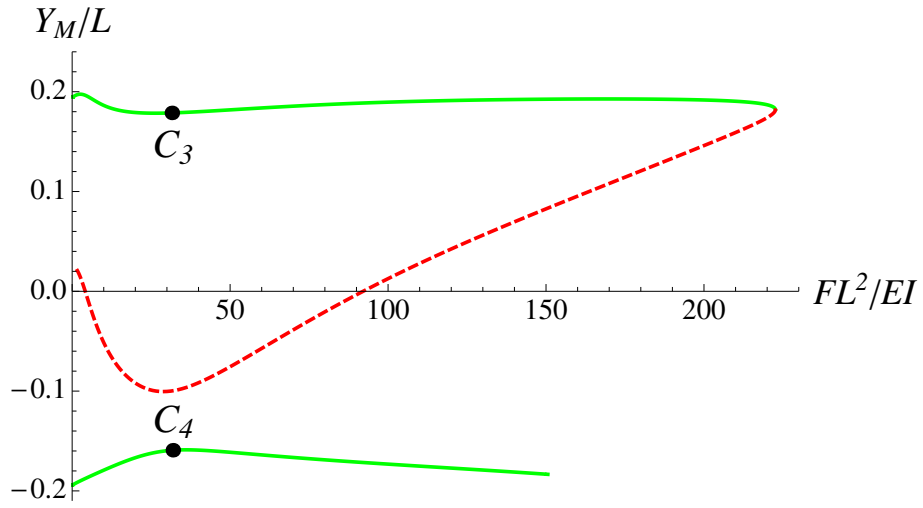

FIG. 4. Bifurcation diagram for  $x_M = 0.48\Delta$  showing  $C_3$  and  $C_4$  configurations that share the same  $F$  value. Plain (respectively dotted) curves correspond to stable (resp. unstable) equilibria.

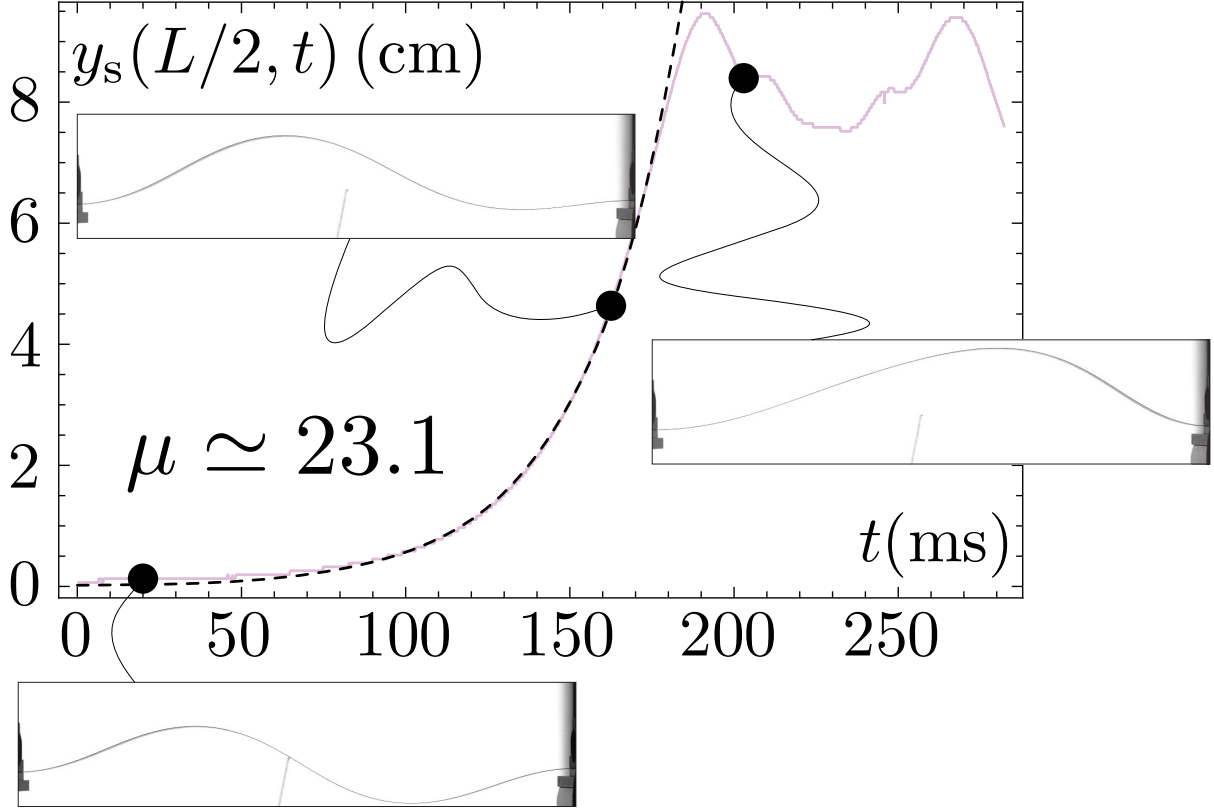

FIG. 5. Position on the beam mid-point  $y_s(L/2, t)$  as function of the physical time  $t$  during a snapping event. Continuous curve corresponds to measured data, while dashed curve is Eq. 1 with fitted  $\mu \simeq 23.1$ .
